# Supplementary material for: The Impact of Human Aspects on the Interactions Between Software Developers and End-Users in Software Engineering: A Systematic Literature Review
Source: arXiv:2405.04787 source file (2024-05-08)
Supplement: Supplementary file 1 [file OnlineAppendix.tex]

%search Strings
\section{Refined Search Strings} \label{Appendix:Refined Search Strings}

\begin{center}
\begin{scriptsize}
\begin{longtable}{ P{0.05\linewidth} P{0.94\linewidth}}
    % \centering
    \caption{Search strings of each database}
    \label{TAB:Search strings of each database}\\
    % \begin{tabular}{ p{0.07\linewidth}  p{0.92\linewidth }}
     % \toprule
     % \hline
     %     \textbf{DB} & \textbf{Final Search String} \\
         % \midrule
    \toprule
    \textbf{DB} & \textbf{Final Search String} \\
    \midrule
    \endfirsthead
    
    \multicolumn{2}{c}%
    {\tablename\ \thetable{} -- \textit{Continued from previous page}} \\
    \midrule
    \textbf{DB} & \textbf{Final Search String} \\
    \midrule
    \endhead
    
    \midrule \multicolumn{2}{r}{\textit{Continued on next page}} \\
    \endfoot
    \bottomrule
    \endlastfoot
         
         IEEE Xplore & (End-User OR End-Users OR End-Customer OR End-Customers OR Software-User OR Software-Users OR User* OR Customer* OR Client*) AND (Developer* OR Software-Developer OR Software-Developers OR Software-Engineer OR Software-Engineers OR Coder* OR Programmer* OR Programer*) AND (Human-Factor OR Human-Factors OR Human-Aspect OR Human-Aspects OR Human-Influence OR Human-Influences OR Human-Issue OR Human-Issues) AND (Interaction OR Relationship OR Involvement OR Association OR Participation) \\
         \midrule
         % \hline
         ACM DL & (``End User" OR ``End Users" OR End-User OR End-Users OR ``End Customer" OR ``End Customers" OR End-Customer OR End-Customers OR ``Software User" OR ``Software Users" OR Customer OR Customers OR User OR Users OR Client OR Clients) AND (Developer OR Developers OR ``Software Developer" OR ``Software Developers" OR ``Software Engineer" OR ``Software Engineers" OR Coder OR Coders OR Programmer OR Programmers OR Programer OR Programers) AND (``Human Factor" OR ``Human Factors" OR ``Human Aspect" OR ``Human Aspects" OR ``Human Influence" OR ``Human Influences" OR ``Human Issue" OR ``Human Issues") AND (Interaction OR Relationship OR Involvement OR Association OR Participation)\\
         \midrule
         % \hline
         Wiley & (``End User" OR ``End Users" OR End-User OR End-Users OR ``End Customer" OR ``End Customers" OR End-Customer OR End-Customers OR ``Software User" OR ``Software Users" OR Customer OR Customers OR User OR Users OR Client OR Clients) AND (Developer OR Developers OR ``Software Developer" OR ``Software Developers" OR ``Software Engineer" OR ``Software Engineers" OR Coder OR Coders OR Programmer OR Programmers OR Programer OR Programers) AND (``Human Factor" OR ``Human Factors" OR ``Human Aspect" OR ``Human Aspects" OR ``Human Influence" OR ``Human Influences" OR ``Human Issue" OR ``Human Issues") AND (Interaction OR Relationship OR Involvement OR Association OR Participation)\\
         \midrule
         % \hline
         TFO & (``End User" OR ``End Users" OR End-User OR End-Users OR ``End Customer" OR ``End Customers" OR End-Customer OR End-Customers OR ``Software User" OR ``Software Users" OR Customer OR Customers OR User OR Users OR Client OR Clients) AND (Developer OR Developers OR ``Software Developer" OR ``Software Developers" OR ``Software Engineer" OR ``Software Engineers" OR Coder OR Coders OR Programmer OR Programmers OR Programer OR Programers) AND (``Human Factor" OR ``Human Factors" OR ``Human Aspect" OR ``Human Aspects" OR ``Human Influence" OR ``Human Influences" OR ``Human Issue" OR ``Human Issues") AND (Interaction OR Relationship OR Involvement OR Association OR Participation)\\
         \midrule
         % \hline
         Springer Link & (``End User" OR ``End-User" OR ``End Customer" OR ``End-Customer" OR ``Software User" OR Customer OR User OR Client) AND (``Developer" OR ``Software Engineer" OR ``Programmer" OR ``Programer" OR ``Coder") AND (``Human Factor" OR ``Human Aspect" OR ``Human Influence" OR ``Human Issue") AND (Interaction OR Relationship OR Involvement OR Association OR Participation)\\
        \midrule
        % \hline
         \multirow[t]{20}{0.05\linewidth}{Science Direct} & (``User" OR ``Customer" OR ``Client") AND (``Developer" OR ``Software Engineer" OR ``Programmer" OR ``Coder") AND (``Human Factor") AND (``Interaction")\\
         & (``User" OR ``Customer" OR ``Client") AND (``Developer" OR ``Software Engineer" OR ``Programmer" OR ``Coder") AND (``Human Factor") AND (``Relationship")\\
         & (``User" OR ``Customer" OR ``Client") AND (``Developer" OR ``Software Engineer" OR ``Programmer" OR ``Coder") AND (``Human Factor") AND (``Involvement") \\
         & (``User" OR ``Customer" OR ``Client") AND (``Developer" OR ``Software Engineer" OR ``Programmer" OR ``Coder") AND (``Human Factor") AND (``Association") \\
         & (``User" OR ``Customer" OR ``Client") AND (``Developer" OR ``Software Engineer" OR ``Programmer" OR ``Coder") AND (``Human Factor") AND (``Participation")\\

         & (``User" OR ``Customer" OR ``Client") AND (``Developer" OR ``Software Engineer" OR ``Programmer" OR ``Coder") AND (``Human Aspect") AND (``Interaction")\\
         & (``User" OR ``Customer" OR ``Client") AND (``Developer" OR ``Software Engineer" OR ``Programmer" OR ``Coder") AND (``Human Aspect") AND (``Relationship")\\
         & (``User" OR ``Customer" OR ``Client") AND (``Developer" OR ``Software Engineer" OR ``Programmer" OR ``Coder") AND (``Human Aspect") AND (``Involvement")\\
         & (``User" OR ``Customer" OR ``Client") AND (``Developer" OR ``Software Engineer" OR ``Programmer" OR ``Coder") AND (``Human Aspect") AND (``Association")\\
         & (``User" OR ``Customer" OR ``Client") AND (``Developer" OR ``Software Engineer" OR ``Programmer" OR ``Coder") AND (``Human Aspect") AND (``Participation")\\

         & (``User" OR ``Customer" OR ``Client") AND (``Developer" OR ``Software Engineer" OR ``Programmer" OR ``Coder") AND (``Human Influence") AND (``Interaction")\\
         & (``User" OR ``Customer" OR ``Client") AND (``Developer" OR ``Software Engineer" OR ``Programmer" OR ``Coder") AND (``Human Influence") AND (``Relationship")\\
         & (``User" OR ``Customer" OR ``Client") AND (``Developer" OR ``Software Engineer" OR ``Programmer" OR ``Coder") AND (``Human Influence") AND (``Involvement")\\
         & (``User" OR ``Customer" OR ``Client") AND (``Developer" OR ``Software Engineer" OR ``Programmer" OR ``Coder") AND (``Human Influence") AND (``Association")\\
         & (``User" OR ``Customer" OR ``Client") AND (``Developer" OR ``Software Engineer" OR ``Programmer" OR ``Coder") AND (``Human Influence") AND (``Participation")\\

         & (``User" OR ``Customer" OR ``Client") AND (``Developer" OR ``Software Engineer" OR ``Programmer" OR ``Coder") AND (``Human Issue") AND (``Interaction")\\
         & (``User" OR ``Customer" OR ``Client") AND (``Developer" OR ``Software Engineer" OR ``Programmer" OR ``Coder") AND (``Human Issue") AND (``Relationship")\\
         & (``User" OR ``Customer" OR ``Client") AND (``Developer" OR ``Software Engineer" OR ``Programmer" OR ``Coder") AND (``Human Issue") AND (``Involvement")\\
         & (``User" OR ``Customer" OR ``Client") AND (``Developer" OR ``Software Engineer" OR ``Programmer" OR ``Coder") AND (``Human Issue") AND (``Association")\\
         & (``User" OR ``Customer" OR ``Client") AND (``Developer" OR ``Software Engineer" OR ``Programmer" OR ``Coder") AND (``Human Issue") AND (``Participation")\\
        
         % \bottomrule
         % \hline
    % \end{tabular}
\end{longtable}
\end{scriptsize}
\end{center}

%Data Extraction Form
\section{Data Extraction Form Fields} \label{Appendix:Data Extraction Form Fields}

\begin{scriptsize}
  \noindent \textbf{General Information:} 
\end{scriptsize}

\begin{enumerate} [1.]
    \scriptsize
    \item Paper ID
    \item Paper title
    \item Authors of the paper
    \item Published year
    \item Venue (Name of the journal/ conference published)
    \item Authors' Affiliation
\end{enumerate}

\begin{scriptsize}
    \noindent \textbf{Key Areas of the Study:} 
\end{scriptsize}

\begin{enumerate} [1.]
\scriptsize
\setcounter{enumi}{6}
    \item Type of Study: Journal Publication/ Conference Paper/ Workshop Paper
    \item Source Type: ACM Digital Library/ IEEE Xplore/ Wiley/ SpringerLink/ ScienceDirect/ Snowballing - Backward/ Snowballing - Forward
    \item What is the motivation/ goals/ objectives of the paper?
    \item What are the Keywords of the paper?
    \item Paper Abstract
    \item Key research questions addressed in the paper
    \item Whose human aspects are analysed in the study: Developers/ End Users/ Other
    \item What are the human aspects considered in the study: Communication/ Perception/ Collaboration/ Emotions/ Human values/ Motivation/ Culture/ Other
    \item What are the definitions used for each of the studied human aspects?
    \item What phases of the SE are considered in the study: Planning/ Requirement Elicitation/ Design Phase/ Development Phase/ Testing Phase/ Maintenance Phase/ Unspecified/ Other
    \item Does the study identify the most affected SE phase by human aspects: Yes/No
    \item If Yes, what is/are the most affected SE phases: Planning/ Requirement Elicitation/ Design Phase/ Development Phase/ Testing Phase/ Maintenance Phase/ Other
\end{enumerate}

\begin{scriptsize}
    \noindent \textbf{Research Methodology:} 
\end{scriptsize}

\begin{enumerate} [1.]
\scriptsize
\setcounter{enumi}{18}
    \item How many participants are considered for the study?
    \item Who are the participants considered for the study (i.e. subset of  `developers' and `stakeholders' eg. `requirements engineers' and `end-users')?
    \item What is/are the role(s) of the developers in the paper?
    \item What is/are the role(s) of the end-users in the paper?
    \item How do the developers and end-users interact with each other: User Feedback, Via documentation, Direct Meetings between developers \& users, Meetings with customer representatives, Communication in Feature requests via Jira or any similar platform, Communication in Defects via Jira or any similar platform, Via Emails, Via App Reviews, Unclear, Other
    \item Are there any middle people who facilitate user-developer interactions: Yes/ No/ Unspecified
    \item If Yes, explain the roles of the middle people who facilitate user-developer interactions?
    \item Does the study use any existing domain models related to human aspects: Yes/No/ Unspecified/ Other
    \item If Yes, What are the existing domain models used to identify the human aspects? Describe the used models.
    \item If Other, Please explain the reason for selecting ``Other" option (eg: Do they use any other models in the study which are not used to capture human aspects).
    \item What research design methods/data collection methods are used in the study: Case studies/ Document analysis/ Surveys or Reviews/ Interviews/ Modelling or Frameworks/ Observations/ Unspecified/ Other
    \item What is the application domain of the study: Tele-Communication (Telco) Software/ Financial Software/ Travel \& Tourism Software/ ERP Applications/ Field service management/ Aviation/ Inventory Management/ AI/ Unspecified/ Other
    \item Is the study conducted based in Academia or Industry: Academia/ Industry/ Mixed/ Unspecified
    \item What type of data analysis used in the study: Quantitative/ Qualitative/ Mixed/ Other
\end{enumerate}

\begin{scriptsize}
    \noindent \textbf{Research Gaps, Limitations \& Future Work:} 
\end{scriptsize}

\begin{enumerate} [1.]
\scriptsize
\setcounter{enumi}{32}
 \item What are the main limitations of the study?
 \item What are the key research gaps/ future work identified by each study?
\end{enumerate}

\begin{scriptsize}
    \noindent \textbf{Research Findings:} 
\end{scriptsize}

\begin{enumerate} [1.]
\scriptsize
\setcounter{enumi}{34}
    \item Does the research include how the human aspect(s) impact on SE field: Yes/ No/ Unspecified
    \item If Yes, what is the nature of the impact of the human aspect(s) on SE: Positive/ Negative/ Undetermined/ Mixed
    \item If Positive, does the study mention the benefits of promoting the human aspect(s)?
    \item If Negative, how it will impact on SE?
    \item Does the study suggest any approach to mitigate the negative impact? Explain.
    \item If Undetermined/Mixed or Other, explain the what kind of impact is there on SE?
    \item Does the research focus on identifying the relationship between different human aspect(s)?
    \item If Yes, what are the identified relationships between different human aspect(s)?
    \item Main outcome/ Results of the study?
    \item Does the study come up with any framework/ model/theory/a set of guidelines as the final outcome: Yes/ No/ Other
    \item If Yes, explain the developed framework/ model/theory/a set of guidelines?
    \item How do they evaluate their results/ framework/ model?
    \item What are the major recommendations of the study?
\end{enumerate}

% Positive effects

\section{Positive Effects of Human Aspects} \label{Appendix:Positive Effects of Human Aspects}

\begin{scriptsize}
\begin{center}
\begin{ThreePartTable}
\begin{TableNotes}
    \item *P: Positive, M: Mixed, UPI: User Participation and Involvement, Challenges: Interpersonal and Intrapersonal Challenges
\end{TableNotes}

\begin{longtable}{P{0.05\linewidth} P{0.09\linewidth} P{0.13\linewidth} P{0.3\linewidth} P{0.35\linewidth}}
% \centering
    \caption{Categorisation of Positive Effects by Human Aspects}
    \label{TAB:Categorisation of Positive Effects by Human Aspects}\\
    
    % \begin{tabular}{P{0.02\linewidth} P{0.07\linewidth} P{0.08\linewidth} P{0.3\linewidth} P{0.35\linewidth} P{0.07\linewidth}}

%     \toprule
%     \textbf{Category} & \textbf{Human Aspect} & \textbf{Nature of Impact} & \textbf{Impact on User-Developer Interactions} & \textbf{Impact on SE} & \textbf{Paper IDs} \\
%     \midrule

    \toprule
    \textbf{Category} & \textbf{Human Aspect} & \textbf{Nature of Impact \& Paper IDs} & \textbf{Impact on User-Developer Interactions} & \textbf{Impact on SE} \\
    \midrule
    \endfirsthead
    
   \multicolumn{3}{r@{}}{{\tablename\ \thetable{} -- \textit{Continued from previous page}}} \\
    \midrule
    \textbf{Category} & \textbf{Human Aspect} & \textbf{Nature of Impact \& Paper IDs} & \textbf{Impact on User-Developer Interactions} & \textbf{Impact on SE}\\
    \midrule
    \endhead
    
    \bottomrule
    \insertTableNotes
    % {\textit{Continued on next page}} \\
    \endfoot
    
    \bottomrule
    \insertTableNotes
    \endlastfoot
    
     % \multirow{8}{*}{\rotatebox[origin=c]{90} {\parbox[c]{1.2cm}{Individual}}} & Empathy & *P: SPR03, SBF08  & Higher level of developer empathy towards users and their needs. & \makecell[tl]{Increased system usability.\\ Enhanced understanding of usability.\\ Resource savings.}\\

     \multirow{8}{*}{\rotatebox[origin=c]{90} {\parbox[c]{1.2cm}{Individual}}} & Empathy & *P:SPR03, SBF08  & Higher level of developer empathy towards users and their needs. & Increased system usability, Enhanced understanding of usability, Resource savings.\\
    
     & Motivation  & \makecell[tl]{P:IEEE02, \\SBB12, SBB01.\\ *M:CHASE02}   & Developer empowerment, Improved developer motivation.  & Improved project success, Improved user commitment to the project. \\
     
     & Perception & \makecell[tl]{P:SBF06. \\M:SBB05}  & Reduced perception gap, Improved client cooperation. & Successful client involvement in software projects. \\
     
     & Emotions & \makecell[tl]{P:ACM01. \\M:IEEE04}  & Quality developer-user relationship due to understanding how users \& developers express emotions, Increased customer satisfaction. & Increasing productivity, Contributing to research of human factors, Improved requirement quality.  \\
     
     & Personality & P:SBB12 &  - & Resolution of complex SE problems by acknowledging individual personality and organisational culture.  \\
     
     & Attitude & P:IEEE02 & - & Better understanding on the impact of Attitude on Engagement.  \\
     
     & Cognitive Style & \makecell[tl]{P:IEEE01, \\SBB04.\\ M:IEEE04, \\WILEY01.} & Reduced understanding gap between customers \& developers. & Increased UPI in decisions about Software, More democratic organisational culture, Improved understanding of problem domain, Quality requirements.  \\
     
     & Competence & P:IEEE02, SBB01 & - & Better understanding of the impact of competence on engagement, Improved user commitment to project team.  \\
   
     \midrule
     \multirow{4}{*}{\rotatebox[origin=c]{90} {\parbox[c]{3cm}{Skill, Experiential or Environmental- influenced}}} & Human Values & \makecell[tl]{P: ACM01, \\SBB12. \\M: IEEE04} & Communication \& trust relationships between users \& developers. & Enhanced understanding on developer thought process, Contributing to research of human factors, Improved customer relations.  \\
    
     & Knowledge & \makecell[tl]{P: SBB04. \\M: IEEE04, \\WILEY01} & Increased knowledge sharing between employees, Effective project requirements definition. & Quality requirements, Increased customer satisfaction, Leading to better systems.  \\
     
     & Skills & M: WILEY01 & - & Supports successful implementation of the SPI efforts.  \\
     
     & Performance & \makecell[tl]{P: SBB01. \\M: SBB02, SBB05} & - & Increased project performance. \\
    
     \midrule
     
     \multirow{6}{*}{\rotatebox[origin=c]{90} {\parbox[c]{2cm}{Group Related}}} & Communication & \makecell[tl]{P: CHASE01, \\ACM01, SD01, \\SPR02, IEEE05, \\IEEE01, SBB09, \\SBB10, SBB13, \\SBB15, SBB14, \\SBB18, SBF01, \\SBF02 SBF04, \\SBF05, SBF10, \\IEEE02, SBB12\\ M:  SBB05, \\SBF07, IEEE04} & Enable a richer communication, Developing and maintaining a strong rapport, Improved developer understanding on user needs, Increased user-developer coordination, Promotes users' positive attitude towards the system, Enables users to use the system more effectively, Facilitate better information flow for users, Increased efficiency of work, Improved opportunities for learning, Improved buy-in and ownership, Improved productivity. & 
     Improved SW \& data quality, Increased system success, Increased user satisfaction, Increased team productivity \& satisfaction, Better UX, Improved system usability, Increased project performance, Quality requirements, Contributing to human factors research, Assisting in guiding \& justifying decision making, Encouraging users to reflect on their use of technology, Reduced defect rate, Reduced utilisation of resources. \\
    
     & Collaboration & \makecell[tl]{P:SD01, IEEE06, \\SBB07, SBB10, \\SBF03, SBF04, \\SBF05, IEEE02, \\SBB12, SBB01\\  M:SBB02,SBB05, \\WILEY01} & Increased collaboration, Increased collaboration between management \& developers, Improved Buy-in \& ownership, Better developer-customer understanding, Reduced conflicts, Increased communication \& coordination, Increased developer appreciation, Improved awareness on user participation \& collaboration, Improved technical, soft, \& project management skills of developers. & Improved system usability, Assisting \& guiding decision making, Increased project performance, Increased user satisfaction, Reduced defect rate, Efficient use of resources, Improved partnership, Continuous cooperation between customer \& supplier to acquire in-depth domain knowledge, Improved user engagement, Better understanding on the impact of collaboration w.r.t. other human aspects, Encouraging startup formation.  \\
     
     & Culture & \makecell[tl]{P:SBF10, IEEE02, \\SBB12, SBB04 \\M: SBF07} & Improved understanding of developer-user cultural differences, Improved communication \& interaction, Reduced difficulties, Quality requirements.  & Improved system success, Improved understanding of cultural variability, Resolution of inter-departmental communication problems, Better understanding on the impact of culture, Collaborative customer relationship, Leading to better systems, Improved awareness of communications strategies, Resolution of complex SE problems by relating to culture.  \\
     
     & Coordination & M:SBB05 & Increased communication \& coordination due to collaboration.  & Increased project performance.  \\
     
     & *Challenges & \makecell[tl]{P:IEEE02 \\M:SBB02, \\SBB08} & Reduced developer-user conflicts, Increased awareness of developer-user differences, Improved communication \& understanding. & Reduced developer-user conflicts, Increased project success, Reduced obstacles in system design and development, Better understanding of the impact of challenges on engagement.\\
     
     & Engagement & \makecell[tl]{P:IEEE02,\\SBB01} & Increased UPI, Improved involvement of leadership \& employees, Improved developer-user collaboration. & Increased system success, Supports successful implementation of the SPI efforts, Improved project performance  \\

% \end{tabular}
\end{longtable}
\end{ThreePartTable}
\end{center}
\end{scriptsize}
